# Supplementary material for: AndesVL Technical Report: An Efficient Mobile-side Multimodal Large Language Model
Source: arXiv:2510.11496 source file (2025-12-22)
Supplement: Supplementary file 1 [file agent_appendix.tex]

\begin{figure*}[!ht] 
\vspace{-5mm}
\begin{AIbox}{Prompt in CIBench}
% {\color{blue}\bf Prompt:} \\
% {
%     \textbf{Question:} 
%     Let $R$ be a ring and let $U$ and $V$ be (two-sided) ideals of $R$. Which of the following must also be ideals of $R$?   
   
% }

% \textbf{Error Analysis:} \\
% In crafting its response, the model fails to accurately grasp the concept of an ideal within a ring.
{\color{blue}\bf System Prompt:}

You are an assistant who can utilize external tools.

\texttt{IPythonInterpreter}: It can run Python code in a manner as jupyter notebook. The code must be a valid code that contains only python method.

% \lstset{style=prompt_json}
% \begin{lstlisting}
% \{\`\ IPythonInterpreter\`\: \`\It can run Python code in a manner as jupyter notebook. The code must be a valid code that contains only python method.\`\ \}
% \end{lstlisting}

To use a tool, please response with the following format: \\

\textbf{Thought}: Think what you need to solve, do you need to use tools? \\

\textbf{Action}: The tool name, should be one of \texttt{IPythonInterpreter}. \\

\textbf{Action Input}: The input to the tool that you want to use. \\
\\
The tool will give you response after your response using the following format: \\

\textbf{Response}: the results after call the tool. \\
\\
Therefore DO NOT generate tool response by yourself. \\

Also please follow the guidelines: \\
1. Always use code interpreter to solve the problem. \\
2. The generated codes should always in a markdown code block format. \\
3. The generated codes will be executed in an ipython manner and the results will be cached. \\
4. Your responded code should always be simple and only solves the problem in current step. \\

For example: \\

File url: \texttt{xxxx} \\
\#\#\# Step 1. Load the dataset from the url into a pandas DataFrame named \texttt{df}. \\

\textbf{Thought}: We should use \texttt{pandas} to solve this step. \\
\textbf{Action}: \texttt{IPythonInterpreter} \\
\textbf{Action Input}: 

\lstset{style=prompt_json}
\begin{lstlisting}
import pandas as pd \\
url = "xxxx" \\
data = pd.read\_csv(url) \\
\end{lstlisting}

\textbf{Response}: The code is succeed without any outputs.

Let us begin from here! \\

{\color{blue}\bf User Prompt:} \\

\{Question\}. Please use \{modules\} modules.

\end{AIbox} 
\caption{Prompt used in CIBench}
\label{fig:prompt_of_cibench}
\end{figure*}

\begin{figure*}[!ht] 
\vspace{-5mm}
\begin{AIbox}{Prompt in CIBench}
{\color{blue}\bf System Prompt:}

You are an assistant who can utilize external tools. \\
\{tool\_description\} \\
To use a tool, please use the following format: \\

\lstset{style=prompt_json}
\begin{lstlisting}
\{thought\}Think what you need to solve, do you need to use tools? \\
\{action\}the tool name, should be one of [\{action\_names\}] \\
\{action\_input\}the input to the action \\
\end{lstlisting}

The response after utilizing tools should using the following format: \\

\lstset{style=prompt_json}
\begin{lstlisting}
\{response\}the results after call the tool. \\
\end{lstlisting}

If you already know the answer, or you do not need to use tools, \\
please using the following format to reply: \\

\lstset{style=prompt_json}
\begin{lstlisting}
\{thought\}the thought process to get the final answer \\
\{finish\}final answer \\
\end{lstlisting}

Begin! \\

{\color{blue}\bf Few-shot Prompt:} \\

\textbf{HUMAN}: Find the coefficient of $x^3$ when $3(x^2 - x^3+x) +3(x +2x^3- 3x^2 + 3x^5+x^3) -5(1+x-4x^3 - x^2)$ is simplifie.

\textbf{BOT}: 

\textbf{Tool}:\texttt{PythonInterpreter}

\textbf{Tool Input}:

\lstset{style=prompt_json}
\begin{lstlisting}
from sympy import symbols, simplify

def solution(): \\
\quad x = symbols('x') \\
\quad expr = $3*(x**2 - x**3 + x) + 3*(x + 2*x**3 - 3*x**2 + 3*x**5 + x**3) - 5*(1 + x - 4*x**3 - x**2)$ \\
\quad simplified\_expr = simplify(expr) \\ 
\quad x3\_coefficient = simplified\_expr.as\_coefficients\_dict()[x**3] \\ 
\quad result = x3\_coefficient \\ 
\quad return result \\
\end{lstlisting}

\textbf{SYSTEM}: Response:26 \\

\textbf{BOT}: FinalAnswer: The final answer is $26$. I hope it is correct. \\
...
\end{AIbox} 
\caption{Prompt used in MATH}
\label{fig:prompt_of_cibench}
\end{figure*}

\begin{figure*}[!ht] 
\vspace{-5mm}
\begin{AIbox}{Prompt in CIBench}
{\color{blue}\bf System Prompt:}

You are an assistant who can utilize external tools. \\
\{tool\_description\} \\
To use a tool, please use the following format: \\

\lstset{style=prompt_json}
\begin{lstlisting}
\{thought\}Think what you need to solve, do you need to use tools? \\
\{action\}the tool name, should be one of [\{action\_names\}] \\
\{action\_input\}the input to the action \\
\end{lstlisting}

The response after utilizing tools should using the following format: \\

\lstset{style=prompt_json}
\begin{lstlisting}
\{response\}the results after call the tool. \\
\end{lstlisting}

If you already know the answer, or you do not need to use tools, \\
please using the following format to reply: \\

\lstset{style=prompt_json}
\begin{lstlisting}
\{thought\}the thought process to get the final answer \\
\{finish\}final answer \\
\end{lstlisting}

Begin! \\

{\color{blue}\bf Few-shot Prompt:} \\

\textbf{HUMAN}: 
Mark's basketball team scores 25 2 pointers, 8 3 pointers and 10 free throws.  Their opponents score double the 2 pointers but half the 3 pointers and free throws.  What's the total number of points scored by both teams added together?

\textbf{BOT}: 

\textbf{Tool}:\texttt{PythonInterpreter}\\

\textbf{Tool Input}: 
\lstset{style=prompt_json}
\begin{lstlisting}
def solution():\\   
mark\_pointers\_2 = 25 * 2   
mark\_pointers\_3 = 8 * 3\\   
mark\_free\_throws = 10 * 1\\   
mark\_points\_scored = mark\_pointers\_2 + mark\_pointers\_3 + mark\_free\_throws\\   
opponents\_pointers\_2 = mark\_pointers\_2 * 2\\   
opponents\_pointers\_3 = mark\_pointers\_3 / 2\\   
opponents\_free\_throws = mark\_free\_throws / 2\\   
opponents\_points\_scored = opponents\_pointers\_2 + opponents\_pointers\_3 + opponents\_free\_throws\\   
total\_points\_scored = mark\_points\_scored + opponents\_points\_scored\\   
result = total\_points\_scored\\   
return result \\
\end{lstlisting}

\textbf{SYSTEM}: Response:201 \\

\textbf{BOT}: Thought: According to the response, I got the answer \\ FinalAnswer: 201 \\

...
\end{AIbox} 
\caption{Prompt used in GSM8K}
\label{fig:prompt_of_agent_gsm8k}
\end{figure*}

% \begin{lstlisting}[style=code]
% # Detect corners using Shi-Tomasi corner detector
% corners = cv2.goodFeaturesToTrack(equalized_image, 
%                                   maxCorners=max_corners, 
%                                   qualityLevel=quality_level, 
%                                   minDistance=min_distance, 
%                                   blockSize=block_size)
% # Mark the corners with circles on the image
% marked_image = equalized_image.copy()
% for corner in corners:
%     x, y = corner.ravel()
%     cv2.circle(marked_image, (int(x), int(y)), 5, (255, 0, 0), -1)  # Draw a blue filled circle at each corner

% # Show the marked image
% plt.imshow(marked_image, cmap='gray')
% plt.axis('off')  # Turn off axis numbers and ticks
% plt.show()

% \end{lstlisting}
